# Supplementary material for: Query Performance Prediction using Relevance Judgments Generated by Large Language Models
Source: arXiv:2404.01012 source file (2025-05-26)
Supplement: Supplementary file 1 [file 09_Appendix.tex]

\section{Appendix}
\subsection{Collection statistics and \ac{IR} performance}
